# Supplementary material for: ComboShoppingBench: Evaluating LLM Agents for Budget-Constrained Basket Shopping with Coupons
Source: arXiv:2608.09282 source file (2026-08-10)
Supplement: Supplementary file 1 [file AnonymousSubmission2027_appendix_labels.tex]

% Fallback cross-document labels for a clean build of AnonymousSubmission2027.tex.
% The main document loads this file only when AnonymousSubmission2027_appendix.aux
% is unavailable.  Keep these section letters in sync if the appendix sections
% are reordered; compiling the appendix locally takes precedence automatically.
\newlabel{app:benchmark-details}{{A}{1}}
\newlabel{app:environment}{{B}{3}}
\newlabel{app:coupon-details}{{C}{5}}
\newlabel{app:construction-details}{{D}{6}}
\newlabel{app:inference-details}{{E}{7}}
\newlabel{app:human-eval}{{F}{7}}
\newlabel{app:more-analysis}{{G}{7}}
\newlabel{app:response-tool-statistics}{{G.1}{7}}
\newlabel{app:prompts}{{H}{9}}
